# Supplementary material for: Anomalous Phase Shift of Quantum Oscillations in 3D Topological Semimetals
Source: arXiv:1604.01681 source file (2016-08-16)
Supplement: Supplementary file 1 [file Weylosci_supp_20160721.pdf]

# Supplemental Material for
# "Anomalous Phase Shift of Quantum Oscillations in 3D Topological Semimetals"

C. M. Wang,[1,2] Hai-Zhou Lu,[1,*] and Shun-Qing Shen[3]

[1] *Department of Physics, South University of Science and Technology of China, Shenzhen 518055, China*
[2] *School of Physics and Electrical Engineering, Anyang Normal University, Anyang 455000, China*
[3] *Department of Physics, The University of Hong Kong, Pokfulam Road, Hong Kong, China*

(Dated: August 3, 2016)

In this Supplemental Material, we present (S1) A survey of the recent experiments on the quantum oscillation in topological semimetals; (S2) An introduction of the calculation procedure for the conductivity and resistivity in the $x$ and $z$ directions under a $z$-direction magnetic field; (S3) The phase shift of the transverse magnetoresistivity for arbitrary $\mu B$; (S4) The quantization rule and phase shift at the Lifshitz point.

## CONTENTS

S1. A survey of the phase shift of the quantum oscillation in experiments S1

S2. The calculation of the resistivity S1
  A. Weyl semimetal without time reversal symmetry S1
  B. Dirac semimetal or Weyl semimetal with time reversal symmetry S2
  C. Numerical scheme S3

S3. Phase shift of resistivity $\rho_{xx}$ for arbitrary $\mu B$ S3

S4. Quantization rule and phase shift at Lifshitz point S5

References S5

## S1. A SURVEY OF THE PHASE SHIFT OF THE QUANTUM OSCILLATION IN EXPERIMENTS

See Table S1 for a survey of the phase shift of the quantum oscillation collected from the recent experiments.

TABLE S1. The oscillation of the magnetoresistance for 3D systems can be phenomenologically fitted by the Lifshitz-Kosevich formula [1, 2] $\Delta\rho \propto \cos 2\pi(F/B+\phi)$ with $F$ the oscillation frequency and $\phi$ the phase shift. This table shows the phase shift $\phi$ of magnetoresistance measured in the experiments. F# distinguishes different frequencies in the samples. S# means different samples. **B** and ***I*** mean the magnetic field and current directions, respectively. c and a are crystallographic axes. T means transverse configuration.

| Ref. | Sample | **B** | ***I*** | $\phi$ |
|---|---|---|---|---|
| [3] | TaAs (F1) | c | a | ≈0 |
| [3] | TaAs (F2) | c | a | -0.96 |
| [4] | TaAs (S1) | c | a | -0.05 |
| [4] | TaAs (S9) | c | a | -0.03 |
| [4] | TaAs (S11) | c | a | 0.02 |
| [4] | TaAs (S14) | c | a | 0.09 |
| [5] | TaP (F1) | c | a | -0.3958 |
| [6] | NbAs | - | - | 0.119 |
| [7] | NbAs (F$\beta$) | c | b | 0.12 |
| [8] | NbP (S1) | - | a | -0.29±0.02 |
| [8] | NbP (S2-2K) | - | a | -0.38±0.03 |
| [8] | NbP (S2-3.3K) | - | a | -0.35±0.03 |
| [8] | NbP (S2-10K) | - | a | -0.31±0.02 |
| [8] | NbP (S7) | - | a | -0.27±0.02 |
| [8] | NbP (S8) | - | a | -0.35±0.04 |
| [8] | NbP (S3)[a] | - | a | -0.31±0.05 |
| [8] | NbP (S4)[b] | - | a | -0.38±0.03 |
| [9] | $Cd_3As_2$ (SA) | T | T | 0.08±0.01 |
| [9] | $Cd_3As_2$ (SB) | T | T | 0.06±0.03 |
| [10] | $Cd_3As_2$ (S2) | [112] | [1$\bar{1}$0] | 0.3 |
| [10] | $Cd_3As_2$ (S2) | [44$\bar{1}$] | [1$\bar{1}$0] | 0.2 |
| [10] | $Cd_3As_2$ (S2) | [112][c] | [1$\bar{1}$0] | 0.38 |
| [10] | $Cd_3As_2$ (S3) | [112] | [1$\bar{1}$0] | 0.11 |
| [11] | $Cd_3As_2$ ($S_1^\alpha$) | T | T | 0.04 |

[a] The Seebeck effect
[b] The Nernst effect
[c] Measured using pulsed magnetic fields

## S2. THE CALCULATION OF THE RESISTIVITY

### A. Weyl semimetal without time reversal symmetry

We calculate the resistivities in both the longitudinal and transverse configurations. In the longitudinal configuration, the electric field is parallel to the magnetic field along the $z$ direction, the resistivity

$$\rho_{zz} = \frac{1}{\sigma_{zz}}. \tag{S1}$$

* luhz@sustc.edu.cn

In the transverse configuration, the electric field is perpendicular to the magnetic field, the resistivity

$$\rho_{xx} = \frac{\sigma_{yy}}{\sigma_{yy}^2 + \sigma_{yx}^2}. \tag{S2}$$

When $\mu B \gg 1$, the nondiagonal conductivity $\sigma_{yx} \approx \sigma_H$, where the Hall conductivity $\sigma_H$ has two parts

$$\sigma_H = \frac{ne}{B} + \frac{e^2}{h}\frac{k_w}{\pi}. \tag{S3}$$

The first term is the classical one with $-e$ the electron charge and $n$ the carrier density measured from the Weyl nodes, and the second term is the anomalous Hall conductance because the two-node model breaks time-reversal symmetry. We numerically evaluate $n$ by using $n = \sum_{\mathbf{k}} f(E_+^{\mathbf{k}})$ for electron carriers. For a Dirac semimetal, there is no anomalous Hall conductance if the Zeeman energy is ignorable. The nondiagonal conductivity $\sigma_{yx}$ for general $\mu B$ also has an oscillation part (see Sec. S3).

The conductivity $\sigma_{zz}$ and $\sigma_{yy}$ take the forms [12, 13]

$$\begin{aligned}\sigma_{zz} &= \frac{e^2}{k_B T}\sum_{\zeta} \tau_\zeta f(E_\zeta)[1-f(E_\zeta)] v_{z\zeta}^2, \\ \sigma_{yy} &= \frac{e^2}{2k_B T}\sum_{\zeta\zeta'} w_{\zeta\zeta'} f(E_\zeta)[1-f(E_{\zeta'})](y_\zeta - y_{\zeta'})^2,\end{aligned} \tag{S4}$$

where $\zeta$ represents all the quantum numbers, $f(E) = 1/\{\exp[(E-E_F)/k_B T]+1\}$ is the Fermi distribution function with $E_F$ the Fermi energy.

$$v_{z\zeta} = \int d\mathbf{r} \Psi_\zeta^\dagger(\mathbf{r}) \hat{v}_z \Psi_\zeta(\mathbf{r}) \tag{S5}$$

is the diagonal matrix element of the velocity operator $\hat{v}_z = \partial\mathcal{H}/\partial\hbar k_z$, and $\Psi$ is the wave function of the Landau levels [14]. The expectation value of the position $y_\zeta = \int d\mathbf{r}\Psi_\zeta^\dagger(\mathbf{r}) y \Psi_\zeta(\mathbf{r})$. The transport relaxation time $\tau_\zeta$ can be found by

$$\frac{1}{\tau_\zeta} = \sum_{\zeta'} w_{\zeta\zeta'}\left(1 - \frac{v_{\mu\zeta'}}{v_{\mu\zeta}}\right), \tag{S6}$$

where the transition rate

$$w_{\zeta\zeta'} = \frac{2\pi}{\hbar}\langle|\langle\Psi_\zeta|V(\mathbf{r})|\Psi_{\zeta'}\rangle|\rangle_{\text{imp}}^2 \delta(E_\zeta - E'_\zeta), \tag{S7}$$

and $\langle\ldots\rangle_{\text{imp}}$ means the averaging over impurity configurations. We consider the elastic impurity scattering with the potential $V(\mathbf{r}) = \sum_{\mathbf{R}_i} U(\mathbf{r}-\mathbf{R}_i)$, and impurities randomly distributing at positions $\mathbf{R}_i$.

For the Landau bands used in this work, we arrive at the transition rate

$$\begin{aligned}w_{\zeta\zeta'} = \frac{2\pi n_{\text{i}}}{\hbar}\sum_{\mathbf{q}} |u(\mathbf{q})|^2 |C_{\zeta\zeta'}(s)|^2 \delta(E_\zeta - E'_\zeta) \\ \times \delta_{k'_x+q_x,k_x}\delta_{k'_z+q_z,k_z},\end{aligned} \tag{S8}$$

where $u(\mathbf{q})$ is the Fourier transform of $U(\mathbf{r})$ with $\mathbf{q}$ wave vector, $n_{\text{i}}$ is the impurity density, and the form factor $|C_{\zeta\zeta'}(s)|^2$ is found as

$$\begin{aligned}|C_{\zeta\zeta'}(s)|^2 = s^{\nu_2-\nu_1} e^{-s}\frac{\nu_1!}{\nu_2!}\Bigg[\sqrt{\frac{\nu_2}{\nu_1}}\sin\theta_\zeta \sin\theta_{\zeta'} \\ \times L_{\nu_1-1}^{\nu_2-\nu_1}(s) + \cos\theta_\zeta\cos\theta_{\zeta'} L_{\nu_1}^{\nu_2-\nu_1}(s)\Bigg]^2,\end{aligned} \tag{S9}$$

with $L_{m_1}^{m_2}(z)$ being associated Laguerre polynomials, $s = \ell_{\text{B}}^2(q_x^2+q_y^2)/2$, $\nu_1 = \min(\nu,\nu')$, $\nu_2 = \max(\nu,\nu')$, $\tan\theta_{\pm\nu k_z} = \left(-\mathcal{M}_{\nu k_z} \pm \sqrt{\mathcal{M}_{\nu k_z}^2 + \nu\eta^2}\right)/\eta\sqrt{\nu}$, $\nu$ denoting the Landau index, $\mathcal{M}_{\nu k_z} = \nu\omega_c + M(k_z^2 - k_w^2)$, $\omega_c = 2M/\ell_B^2$, $\eta = A\sqrt{2}/\ell_B$, and the magnetic length $\ell_B = \sqrt{\hbar/|eB|}$.

### B. Dirac semimetal or Weyl semimetal with time reversal symmetry

For the model of Dirac semimetals [14, 15], the conductivities $\sigma_{zz}$ and $\sigma_{yy}$ are the same as Eq. (S4) except for an additional branch index from different partners in $\zeta$. If we label the previous branch as partner 1, the second branch from the time-reversal partner $\mathcal{H}^*(-\mathbf{k})$ is labeled as partner 2. The intrabranch form factor of the first partner $|C_{\zeta\zeta'}(s)|^2$ is rewritten as $|C_{\zeta\zeta'}^{11}(s)|^2$. The intrabranch form factor of the second partner $|C_{\zeta\zeta'}^{22}(s)|^2$ is obtained by interchanging $\cos\theta_\zeta$ and $\cos\theta_{\zeta'}$ with $\sin\theta_\zeta$ and $\sin\theta_{\zeta'}$ in $|C_{\zeta\zeta'}^{11}(s)|^2$. The interbranch form factor between two partners $|C_{\zeta\zeta'}^{12}(s,\varphi)|^2$ is also related to the angle $\varphi = \tan^{-1}(q_y/q_x)$, and is given by

$$|C^{12}_{\zeta\zeta'}(s,\varphi)|^2 = e^{-s}\Big\{ s^{\nu_{a2}-\nu_{a1}} \sin^2\theta_\zeta \sin^2\theta_{\zeta'} \left(L^{\nu_{a2}-\nu_{a1}}_{\nu_{a1}}\right)^2 \frac{\nu_{a1}!}{\nu_{a2}!} + s^{\nu_{b2}-\nu_{b1}} \cos^2\theta_\zeta \cos^2\theta_{\zeta'} \left(L^{\nu_{b2}-\nu_{b1}}_{\nu_{b1}}\right)^2 \frac{\nu_{b1}!}{\nu_{b2}!}$$
$$+ \frac{1}{2}\tau_1^{\nu_{a2}-\nu_{a1}} \tau_2^{\nu_{b2}-\nu_{b1}} s^{(\nu_{a2}+\nu_{b2}-\nu_{a1}-\nu_{b1})/2} \sin 2\theta_\zeta \sin 2\theta_{\zeta'} \cos[\tau_1(\nu_{a2}-\nu_{a1})\varphi - \tau_2(\nu_{b2}-\nu_{b1})\varphi]$$
$$\times L^{\nu_{a2}-\nu_{a1}}_{\nu_{a1}} L^{\nu_{b2}-\nu_{b1}}_{\nu_{b1}} \sqrt{\frac{\nu_{a1}!}{\nu_{a2}!}} \sqrt{\frac{\nu_{b1}!}{\nu_{b2}!}} \Big\} \tag{S10}$$

.

Here

$$\tau_1 = \begin{cases} +1, & \nu < \nu'+1, \\ -1, & \nu > \nu'+1, \end{cases} \tag{S11}$$

$$\tau_2 = \begin{cases} +1, & \nu < \nu'-1, \\ -1, & \nu > \nu'-1, \end{cases} \tag{S12}$$

and $\nu_{a1} = \min(\nu-1,\nu')$, $\nu_{a2} = \max(\nu-1,\nu')$, $\nu_{b1} = \min(\nu,\nu'-1)$, $\nu_{b2} = \max(\nu,\nu'-1)$. The other interbranch form factor $|C^{21}_{\zeta\zeta'}(s,\varphi)|^2$ can be obtained by interchanging $\cos\theta_\zeta$ and $\cos\theta_{\zeta'}$ with $\sin\theta_\zeta$ and $\sin\theta_{\zeta'}$ in $|C^{12}_{\zeta\zeta'}(s,\varphi)|^2$.

### C. Numerical scheme

In this work, we consider the electron conduction case at zero temperature and assume short-range scattering $u(\boldsymbol{q}) = u_0$. In the presence of the $z$-direction magnetic field, we numerically calculate the resistivity $\rho_{zz}$ in the longitudinal configuration and $\rho_{xx}$ in the transverse configuration, with the formulas above.

In the presence of disorder, the Landau bands are broadened, inevitably. A Gaussian form broadening is modeled with a constant width $\Gamma$. Hence, $\delta(E_\zeta - E_F)$ is replaced by

$$\delta(E_\zeta - E_F) \rightarrow \sqrt{\frac{2}{\pi\Gamma^2}} \exp\left[-\frac{2(E_\zeta - E_F)^2}{\Gamma^2}\right]. \tag{S13}$$

In the calculation, the broadening width $\Gamma$ is taken to be the energy interval between the valleys of $E^{k_z}_{+16}$ and $E^{k_z}_{+15}$. The scattering potential $n_i u_0^2 = 3\pi A^3\Gamma/E_F^2\alpha_\Gamma$, with $\alpha_\Gamma = 10$ a phenomenological parameter that relates the electron lifetime to the transport scattering time.

To eliminate the non-oscillation background, the third-order derivative of the resistivity with respect to $B$ are evaluated. Therefore, the peaks and valleys of $\rho_{xx}$ correspond to the zeros of $d^3\rho_{xx}/dB^3$. By assigning the peaks and valleys of resistivity to be integer and half-integer indices, respectively, one obtains the Landau index plot. The slope and intercept of the plot give the oscillation frequency and the phase shift, respectively. In order to get continuous curves of the phase shift, one has to choose a gauge in which the intercept $\phi = -1/8, -5/8$ when $E_F \rightarrow 0$ and $\infty$, respectively, for electron carriers.

## S3. PHASE SHIFT OF RESISTIVITY $\rho_{xx}$ FOR ARBITRARY $\mu B$

For arbitrary $\mu B$, especially $\mu B \approx 1$ with $\mu$ the mobility, one has to consider the oscillation of the nondiagonal (Hall) conductivity $\sigma_{yx}$. We will discuss this effect with the help of Green's function formulism [16]. The tensor of the static conductivity is given by

$$\sigma_{\alpha\beta} = \frac{e^2\hbar}{2\pi} \int dE f(E) \mathrm{Tr} \left\langle \left\| \left[ \hat{v}_\alpha \frac{\partial \hat{G}^R}{\partial E} \hat{v}_\beta \left(\hat{G}^A - \hat{G}^R\right) - \left(\hat{G}^A - \hat{G}^R\right) \hat{v}_\beta \frac{\partial \hat{G}^A}{\partial E} \hat{v}_\alpha \right] \right\| \right\rangle_{\mathrm{imp}}, \tag{S14}$$

with $\hat{G}^{R/A}$ being the retarded/advanced Green's function, the velocity operator $\hat{v}_\alpha = \partial\mathcal{H}/\partial\hbar k_\alpha$, where the wave vector should be replaced by $\mathbf{k} = (k_x - eBy/\hbar, -i\partial_y, k_z)$ under the Pierls replacement. The conductivity tensor can be calculated in the Landau band representation. The matrix elements of the velocity operator for electrons are written as

$$v_{x\zeta\zeta'} = \int d\mathbf{r} \Psi^\dagger_\zeta(\mathbf{r}) \hat{v}_x \Psi_{\zeta'}(\mathbf{r}) = v^{(1)}_{\nu'\nu} \delta_{k_x k_x'} \delta_{k_z k_z'} \delta_{n,n'-1} + v^{(2)}_{\nu'\nu} \delta_{k_x k_x'} \delta_{k_z k_z'} \delta_{n,n'+1}, \tag{S15}$$

$$v_{y\zeta\zeta'} = \int d\mathbf{r} \Psi^\dagger_\zeta(\mathbf{r}) \hat{v}_y \Psi_{\zeta'}(\mathbf{r}) = -iv^{(1)}_{\nu'\nu} \delta_{k_x k_x'} \delta_{k_z k_z'} \delta_{n,n'-1} + iv^{(2)}_{\nu'\nu} \delta_{k_x k_x'} \delta_{k_z k_z'} \delta_{n,n'+1}, \tag{S16}$$

with

$$v^{(1)}_{\nu\nu'} = A\hbar^{-1} \sin\theta_{+\nu k_z} \cos\theta_{+\nu' k_z} + \sqrt{2} M \ell_B^{-1} \hbar^{-1} \times \left(\sqrt{\nu-1} \sin\theta_{+\nu k_z} \sin\theta_{+\nu' k_z} - \sqrt{\nu} \cos\theta_{+\nu k_z} \cos\theta_{+\nu' k_z}\right), \tag{S17}$$

$$v^{(2)}_{\nu\nu'} = A\hbar^{-1} \cos\theta_{+\nu k_z} \sin\theta_{+\nu' k_z} + \sqrt{2} M \ell_B^{-1} \hbar^{-1} \times \left(\sqrt{\nu} \sin\theta_{+\nu k_z} \sin\theta_{+\nu' k_z} - \sqrt{\nu+1} \cos\theta_{+\nu k_z} \cos\theta_{+\nu' k_z}\right). \tag{S18}$$

For simplicity, by using a constant broadening $\gamma$, the retarded/advanced Green's function of electrons is given by

$$G_{\nu}^{R/A} = \frac{1}{E - E_{+\nu}^{k_z} \pm i\gamma}, \tag{S19}$$

where the Landau bands $E_{+\nu}^{k_z} = \omega_c/2 + \sqrt{\mathcal{M}_{\nu k_z}^2 + \nu\eta^2}$ for $\nu \geq 1$, $E_0^{k_z} = \omega_c/2 + \mathcal{M}_{0k_z}$ for $\nu = 0$, and $\gamma = \hbar/2\tau$ with $\tau$ the lifetime. Therefore, the diagonal conductivity can be obtained as

$$\sigma_{yy} = -\frac{e^3 B}{\pi^2}\int dE \frac{df(E)}{dE} \times \sum_{\nu,k_z} \frac{v_{\nu+1\nu}^{(1)} v_{\nu\nu+1}^{(2)} \gamma^2}{\left[(E - E_{+\nu}^{k_z})^2 + \gamma^2\right]\left[(E - E_{+\nu+1}^{k_z})^2 + \gamma^2\right]}. \tag{S20}$$

After some transformations, this conductivity can be rewritten as

$$\sigma_{yy} = -\frac{e^3 B}{4\pi^2}\int dE \frac{df(E)}{dE} \times \sum_{\nu,k_z} \frac{v_{\nu+1\nu}^{(1)} v_{\nu\nu+1}^{(2)} (2\gamma)^2}{(E_{+\nu+1}^{k_z} - E_{+\nu}^{k_z})\left[(E_{+\nu+1}^{k_z} - E_{+\nu}^{k_z})^2 + (2\gamma)^2\right]} \times \left[\frac{2E - 3E_{+\nu}^{k_z} + E_{+\nu+1}^{k_z}}{(E - E_{+\nu}^{k_z})^2 + \gamma^2} - \frac{2E - 3E_{+\nu+1}^{k_z} + E_{+\nu}^{k_z}}{(E - E_{+\nu+1}^{k_z})^2 + \gamma^2}\right]. \tag{S21}$$

This expression can be simplified for small broadening

$$\sigma_{yy} \approx -\frac{e^3 B}{4\pi^2}\int dE \frac{df(E)}{dE} \times \sum_{\nu,k_z} \frac{v_{\nu+1\nu}^{(1)} v_{\nu\nu+1}^{(2)} (2\gamma)^2}{\left[(E_{+\nu+1}^{k_z} - E_{+\nu}^{k_z})^2 + (2\gamma)^2\right]} \frac{1}{(E - E_{+\nu+1}^{k_z})^2 + \gamma^2}. \tag{S22}$$

The nondiagonal Hall conductivity $\sigma_{yx}$ is expressed as

$$\sigma_{yx} = \frac{e^3 B}{4\pi^2}\int dE \frac{df(E)}{dE} \sum_{\nu,k_z} L_{\nu,k_z}(E), \tag{S23}$$

with

$$L_{\nu,k_z}(E) = \int_{-\infty}^{E} dE' v_{\nu+1\nu}^{(1)} v_{\nu\nu+1}^{(2)} \times \frac{8\gamma\left[(E' - E_{+\nu+1}^{k_z})^2 (E' - E_{+\nu}^{k_z})^2 - \gamma^4\right]}{\left[(E' - E_{+\nu+1}^{k_z})^2 + \gamma^2\right]^2 \left[(E' - E_{+\nu}^{k_z})^2 + \gamma^2\right]^2}. \tag{S24}$$

After performing the above integral, the nondiagonal conductivity yields a dissipativeless part and a dissipative part,

$$\sigma_{yx} = \sigma_H - \Delta\sigma_{yx}, \tag{S25}$$

where

$$\Delta\sigma_{yx} = -\frac{e^3 B}{4\pi^2}\int dE \frac{df(E)}{dE} \sum_{\nu,k_z} \frac{v_{\nu+1\nu}^{(1)} v_{\nu\nu+1}^{(2)} (2\gamma)}{(E_{+\nu+1}^{k_z} - E_{+\nu}^{k_z})^2 + (2\gamma)^2} \times \left\{ \frac{2\left(E - E_{+\nu+1}^{k_z}\right)}{\left(E - E_{+\nu+1}^{k_z}\right)^2 + \gamma^2} + \frac{(2\gamma)^2}{\left(E_{+\nu+1}^{k_z} - E_{+\nu}^{k_z}\right)\left[\left(E - E_{+\nu+1}^{k_z}\right)^2 + \gamma^2\right]} \right\}. \tag{S26}$$

The first term in the curly braces of $\Delta\sigma_{yx}$ almost vanishes due to the summation over $\nu$. Therefore, according to Eqs. (S22) and (S26), the difference between $\sigma_{yy}$ and $\Delta\sigma_{yx}$ is only a factor $2\gamma/(E_{+\nu+1}^{k_z} - E_{+\nu}^{k_z})$ in the summation. This factor can be approximated as $1/\mu B$, then

$$\sigma_{yx} \sim \sigma_H - \frac{\sigma_{yy}}{\mu B}. \tag{S27}$$

Hence, the oscillation of $\sigma_{yx}$ differs from that of $\sigma_{yy}$ by a $\pi$ phase, and $\Delta\sigma_{yx}$ is in higher orders of $1/\mu B$. This relation is also known for conventional electron gases with parabolic band dispersion [16].

When $\sigma_{yx} \gg \sigma_{yy}$ or $\mu B \gg 1$, which holds in most experiments, the oscillation part of $\sigma_{yx}$ can be abandoned. Hence,

$$\rho_{xx} = \frac{\sigma_{yy}}{\sigma_{yy}^2 + \sigma_{yx}^2} \approx \frac{\sigma_{yy}}{\sigma_{yy}^2 + \sigma_H^2} \approx \frac{\sigma_{yy}}{\sigma_H^2}, \tag{S28}$$

so $\rho_{xx}$ and $\sigma_{yy}$ are in phase.

In fact, $\rho_{xx}$ and $\sigma_{yy}$ are always in phase for any $\mu B$. To see this, for arbitrary $\mu B$, the diagonal conductivity in Eq. (S22) can always be expressed as

$$\sigma_{yy} \sim \frac{\sigma_0(1+\delta)}{1+(\mu B)^2}, \tag{S29}$$

where $\delta \ll 1$ represents the oscillation part and $\sigma_0 = en\mu \approx \mu B \sigma_H$ is the conductivity in the absence of magnetic field (the anomalous part of $\sigma_H$ is suppressed for simplicity). Use Eq. (S27),

$$\sigma_{yx} = \frac{\sigma_0}{\mu B} - \frac{\sigma_{yy}}{\mu B} = \frac{(\mu B)\sigma_0}{1+(\mu B)^2}\left[1 - \frac{\delta}{(\mu B)^2}\right], \tag{S30}$$

and

$$\rho_{xx} = \frac{\frac{\sigma_0(1+\delta)}{1+(\mu B)^2}}{\left[\frac{\sigma_0(1+\delta)}{1+(\mu B)^2}\right]^2 + \left[\frac{(\mu B)\sigma_0}{1+(\mu B)^2}\left(1 - \frac{\delta}{(\mu B)^2}\right)\right]^2} \approx \frac{1+\delta}{\sigma_0}, \tag{S31}$$

up to the leading order of $\delta$. According to Eqs. (S29) and (S31), both $\sigma_{yy}$ and $\rho_{xx}$ are proportional to $\delta$ for arbitrary $\mu B$, so $\rho_{xx}$ is always in phase with $\sigma_{yy}$. When

$\sigma_{yx} \ll \sigma_{yy}$, we have $\rho_{yx} \ll \rho_{xx}$. If the oscillation of $\sigma_{yx}$ is neglected, one could arrive at $\rho_{xx} = \sigma_{yy}/(\sigma_{yy}^2 + \sigma_{yx}^2) = 1/\sigma_{yy}$, it seems that the oscillation of $\rho_{xx}$ differs from that of $\sigma_{yy}$ by a $\pi$ phase. This conclusion is found to be wrong according to above analysis.

## S4. QUANTIZATION RULE AND PHASE SHIFT AT LIFSHITZ POINT

From $E_{+\nu}^{k_z} = E$, the quantization rule is given by

$$2\pi\nu\frac{eB}{\hbar} = \pi\Bigg\{ - \left(k_z^2 - k_w^2 + \frac{k_0^2}{2}\right) \pm \frac{1}{2}\sqrt{k_0^4 + 4k_0^2(k_z^2 - k_w^2) + 4\left(\frac{E - \omega_c/2}{M}\right)^2}\Bigg\}, \quad \text{(S32)}$$

where $k_0 \equiv A/M$. There are two situations. For this 3D case, the Landau indices also depend on the third component of the wave vector, giving a quantization rule that is beyond the Onsager's rule. There are also $B$-dependent terms on the right hand side. The 0th order term of $\omega_c$ leads to the area in the $k_x$-$k_y$ plane by fixing $k_z$ as a parameter; the first order term represents the magnetization; the second order term denotes the magnetic susceptibility, and so on [17]. In contrast to the linear and parabolic limits, due to the complex structure of the energy spectrum, the Landau indices now do not linearly depend on $k_z^2$. Hence, the $-1/8$ phase shift originating from the simple $k_z$ integral in the two limits is changed. As an example, we calculate the total phase shift at the Lifshitz point $E_F = E_M$ when $E_M = E_A$. The oscillation part of the resistivity $\rho_{xx}$ is written as

$$\rho_{xx}^{\text{os}} \propto \sum_{k_z} \int dx \delta(E_{+x}^{k_z} - E_F) \cos(2\pi x). \quad \text{(S33)}$$

When $E_M = E_A$, only the positive branch of Eq. (S32) contributes to the resistivity. After the integration and summation, it is found that

$$\rho_{xx}^{\text{os}} \propto \cos\left[2\pi\left(\frac{E_F}{\eta}\right)^2 + \frac{\pi}{2}\left(\frac{\eta}{E_F}\right)^2 + \alpha\right], \quad \text{(S34)}$$

where

$$\tan\alpha = \frac{1 - 2S(z)}{1 - 2C(z)}, \quad \text{(S35)}$$

with $S(z)$ and $C(z)$ being the Fresnel sine and cosine integrals, $z = \left(\sqrt{\xi^4 - 4\xi^2 + 1} - 1\right)/\xi$, and $\xi = \eta/E_F$. To the lowest order of $\xi$,

$$\rho_{xx}^{\text{os}} \propto \cos\left[2\pi\left(\frac{E_F^2}{\eta^2} - \frac{9}{8} + \mathcal{O}(\xi)\right)\right]. \quad \text{(S36)}$$

The phase shift at the Lifshitz point is a universal value to the lowest order of $\xi$. This is in consistence with the numerical results. This value of the phase shift at the Lifshitz point verifies the non-monotonic behavior of the phase shift as a function of the Fermi energy.


[1] D. Shoenberg, *Magnetic oscillations in metals* (Cambridge University Press, 1984).
[2] H. Murakawa, M. S. Bahramy, M. Tokunaga, Y. Kohama, C. Bell, Y. Kaneko, N. Nagaosa, H. Y. Hwang, and Y. Tokura, Science **342**, 1490 (2013).
[3] X. C. Huang, *et al.*, Phys. Rev. X **5**, 031023 (2015).
[4] C. Zhang, *et al.*, Nat. Commun. **7**, 10735 (2016).
[5] J. Du, *et al.*, Sci. China-Phys. Mech. Astron. **59**, 657406 (2016).
[6] X. Yang, Y. Li, Z. Wang, Y. Zhen, and Z.-a. Xu, arXiv:1506.02283 (2015).
[7] Y. Luo, N. J. Ghimire, M. Wartenbe, H. Choi, M. Neupane, R. D. McDonald, E. D. Bauer, J. Zhu, J. D. Thompson, and F. Ronning, Phys. Rev. B **92**, 205134 (2015).
[8] Z. Wang, *et al.*, Phys. Rev. B **93**, 121112(R) (2016).
[9] L. P. He, X. C. Hong, J. K. Dong, J. Pan, Z. Zhang, J. Zhang, and S. Y. Li, Phys. Rev. Lett. **113**, 246402 (2014).
[10] Y. F. Zhao, *et al.*, Phys. Rev. X **5**, 031037 (2015).
[11] A. Narayanan, *et al.*, Phys. Rev. Lett. **114**, 117201 (2015).
[12] M. Charbonneau, K. M. van Vliet, and P. Vasilopoulos, J. Math. Phys. **23**, 318 (1982).
[13] P. Vasilopoulos and C. Van Vliet, J. Math. Phys. **25**, 1391 (1984).
[14] H. Z. Lu, S. B. Zhang, and S. Q. Shen, Phys. Rev. B **92**, 045203 (2015).
[15] S.-B. Zhang, H.-Z. Lu, and S.-Q. Shen, New Journal of Physics **18**, 053039 (2016).
[16] F. T. Vasko and O. E. Raichev, *Quantum Kinetic Theory and Applications: Electrons, Photons, Phonons* (Springer Science & Business Media, 2006).
[17] Y. Gao and Q. Niu, arXiv:1507.06342 (2015).
